# Supplementary material for: Fine-tuning Image Transformers using Learnable Memory
Source: arXiv:2203.15243 source file (2022-03-30)
Supplement: Supplementary file 1 [file supplemental.tex]

% CVPR 2022 Paper Template
% based on the CVPR template provided by Ming-Ming Cheng (https://github.com/MCG-NKU/CVPR_Template)
% modified and extended by Stefan Roth (stefan.roth@NOSPAMtu-darmstadt.de)

\documentclass[10pt]{article}

%%%%%%%%% PAPER TYPE  - PLEASE UPDATE FOR FINAL VERSION
%usepackage[review]{cvpr}      % To produce the REVIEW version
\usepackage{cvpr}  % To produce the CAMERA-READY version

\usepackage{diagbox}
\usepackage{graphicx}
\usepackage{amsmath}
\usepackage{amssymb}
\usepackage{booktabs}
\usepackage{color}
\usepackage{xcolor}
\usepackage{multirow}
\definecolor{darkgreen}{RGB}{0,127,0}

\newcommand{\TODONE}[1]{}
\usepackage[pagebackref,breaklinks,colorlinks]{hyperref}

% Support for easy cross-referencing
\usepackage[capitalize]{cleveref}
\crefname{section}{Sec.}{Secs.}
\Crefname{section}{Section}{Sections}
\Crefname{table}{Table}{Tables}
\crefname{table}{Tab.}{Tabs.}

%%%%%%%%% PAPER ID  - PLEASE UPDATE
 % *** Enter the CVPR Paper ID here

\definecolor{mplblue}{rgb}{0., 0.5, 0.91}
\begin{document}
%\vspace{-1ex}\paragraph
\input{appendix}
%%%%%%%%% ABSTRACT

\end{document}
